# Supplementary material for: Sleeping Combinatorial Bandits
Source: arXiv:2106.01624 source file (2021-06-03)
Supplement: Supplementary file 1 [file supplimentary.tex]

%%%% ijcai21.tex

\typeout{IJCAI--21 Instructions for Authors}

% These are the instructions for authors for IJCAI-21.

\documentclass{article}
\pdfpagewidth=8.5in
\pdfpageheight=11in
% The file ijcai21.sty is NOT the same than previous years'
%\usepackage{ijcai21}

% Use the postscript times font!
\usepackage{times}
\usepackage{soul}
\usepackage{url}
\usepackage[hidelinks]{hyperref}
\usepackage{float}
\usepackage[utf8]{inputenc}
\usepackage[small]{caption}
\usepackage{graphicx}
\usepackage{amsmath,bbm}
\usepackage{amsthm}
\usepackage{booktabs}
\usepackage{algorithm}
\usepackage{algorithmic}
\urlstyle{same}
\input{macro.tex}
\title{Combinatorial Sleeping Bandits: Supplimentary Material}

\author{ }
\begin{document}
\maketitle
\appendix
\input{appendix.tex}

\end{document}
